# Supplementary material for: The Benefits of Probability-Proportional-to-Size Sampling in Cluster-Randomized Experiments
Source: arXiv:2002.08009 source file (2020-02-19)
Supplement: Supplementary file 1 [file AppendixA-HTSRS.tex]

\cleardoublepage

\section{Properties of the HT-SRS estimator} \label{appendixhtsrs}

We begin by investigating the properties of $\hat\mu_{t,\text{HT,SRS}}$.  Then using these properties, we prove lemma~\ref{HTSRSlemma}.      

\subsection{Useful indicator expectations under SRS}
Let $\mathbf S = (S_1,S_2,\ldots, S_n)$ denote a random set of cluster sampling indicator variables under SRS.  For any distinct clusters $c$ and $c'$ and distinct treatments $t=1$ and $t=0$, the following expectations hold under complete randomization of treatment to units, provided that $S_c =1$ (and when applicable, $S_{c'} =1$): 
\begin{align}
  \E(S_c | \#T_t) ={}& \frac{s}{\ell} \\
  \E(S_cS_{c'} | \#T_t) ={}& \frac{s}{\ell}\frac{s-1}{\ell-1} \\
  \E\left(S_c^2T_{ct}^2|\#T_t\right) ={}& \E\left(S_cT_{ct}|\#T_t\right) = \E\left(S_c \E\left(\left.T_{ct}\right|\mathbf{S}\right)|\#T_t\right) 
  \nn ={}& \frac{\#T_t}{s}\E\left(S_c|\#T_t\right) 
  \nn ={}& \frac{\#T_t}{\ell}  \\
  \E(S_cS_{c'}T_{ct}T_{c't} | \#T_t) ={}& \E(S_cS_{c'}\E(T_{ct}T_{c't} | \mathbf{S}) | \#T_t) 
  \nn ={}& \frac{\#T_t}{s}\frac{\#T_t-1}{s-1} \E(S_cS_{c'} | \#T_t)  
  \nn ={}& \frac{\#T_t(\#T_t-1)}{\ell(\ell-1)} \\
  \E(S_cS_{c'}T_{c1}T_{c'0} | \#T_1, \#T_0) ={}& \E(S_cS_{c'}\E(T_{c1}T_{c'0} | \mathbf{S}) | \#T_1, \#T_0) 
  \nn ={}& \frac{\#T_1}{s}\frac{\#T_0}{s-1} \E(S_cS_{c'}|\#T_1, \#T_0) 
  \nn ={}& \frac{\#T_1\#T_0}{\ell(\ell-1)} \\ \nn
  \E\left(\frac{S_c^2T_{ct}^2}{\#T_t^2} \right) ={}& \E\left(\frac{1}{\#T_t^2} \E(S_c^2T_{ct}^2 |\#T_t) \right) 
  = \frac{1}{\ell}\E\left(\frac{1}{\#T_t} \right) \\
  \var\left(S_cT_{ct} | \#T_t\right) ={}& \frac{\#T_t}{\ell}\left(1-\frac{\#T_t}{\ell} \right) \\
  \var\left(\frac{S_cT_{ct}}{\#T_t}\right) ={}& \var\left(\frac{1}{\#T_t} \E(S_cT_{ct} | \#T_t) \right) + \E\left(\frac{1}{\#T_t^2} \var(S_cT_{ct}|\#T_t) \right)
  \nn ={}& \frac{1}{\ell} \E\left(\frac{1}{\#T_t}\right) - \frac{1}{\ell^2} \\
  \cov\left(\frac{S_cT_{ct}}{\#T_t}, \frac{S_{c'}T_{c't}}{\#T_t}\right) ={}& \cov\left(\frac{1}{\#T_t}\E(S_cT_{ct}|\#T_t), \frac{1}{\#T_t}\E(S_{c'}T_{c't}|\#T_t) \right)
  \nn {}& + \E\left(\frac{1}{\#T_t^2}\cov(S_cT_{ct}, S_{c'}T_{c't} | \#T_t) \right)
  \nn ={}& \E\left(\frac{1}{\#T_t^2} \Bigg[\E(S_cS_{c'}T_{ct}T_{c't} | \#T_t) - \E(S_cT_{ct}|\#T_t)\E(S_{c'}T_{c't}|\#T_t)\Bigg] \right) \nn ={}& \frac{1}{\ell(\ell-1)}\E\left(1-\frac{1}{\#T_t}\right)-\frac{1}{\ell^2} \\
  \var\left(\frac{S_cT_{c1}T_{c'0}}{\#T_1\#T_0}\right) ={}& \E\left(\frac{1}{\#T_1\#T_0} \E(S_c^2T_{c1}T_{c'0}|\#T_1, \#T_0)\right) 
  \nn {}& - \E\left(\frac{1}{\#T_1}\E(S_cT_{c1}|\#T_1)\right)\E\left(\frac{1}{\#T_0}\E(S_cT_{c0}|\#T_0)\right)
  \nn ={}& - \frac{1}{\ell^2} \\
  \cov\left(\frac{S_cT_{c1}}{\#T_1}, \frac{S_{c'}T_{c'0}}{\#T_0}\right) ={}& \E\left(\frac{1}{\#T_1\#T_0} \E(S_cS_{c'}T_{c1}T_{c'0}|\#T_1, \#T_0)\right) 
  \nn {}& - \E\left(\frac{1}{\#T_1}\E(S_cT_{c1}|\#T_1)\right) \E\left(\frac{1}{\#T_0} \E(S_{c'}T_{c'0}|\#T_0)\right)
  \nn ={}& \frac{1}{\ell(\ell-1)} - \frac{1}{\ell^2}
\end{align}

Conditional on the sampled clusters, units are sampled within a cluster using simple random sampling, and this secondary sampling stage is independent of cluster treatment assignment.  Thus, the expectation of within-cluster sampling indicators are independent of the cluster treatment indicators.  Moreover, within-cluster samples are drawn independently across clusters, and so for distinct units $k$ and $k'$ in the same cluster $c$ or distinct units $k$ and $k^*$ in different clusters $c$ and $c'$:
 \begin{align} 
        \E\left( S_{kc} | \mathbf S \right) &=  \frac{s_c}{n_c}  \label{unitsampexp1}\\
        \E\left( S_{kc}S_{k'c} | \mathbf S\right) &=  \frac{s_c(s_c - 1)}{n_c(n_c - 1)}   \\
        \E\left( S_{kc}S_{k^*c'} | \mathbf S\right) &= \frac{s_cs_{c'}}{n_c n_{c'}}  \\
        \var(S_{kc}| \mathbf S) &= \frac{s_c}{n_c}\left(1-\frac{s_c}{n_c}\right) \\
        \cov(S_{kc}, S_{k'c}| \mathbf S) &= \E(S_{kc}S_{k'c}| \mathbf S)- \E(S_{kc}| \mathbf S)\E(S_{k'c}| \mathbf S)
        \nn &= -\frac{s_c}{n_c}\frac{1}{n_c-1}\left(1-\frac{s_c}{n_c}\right) \label{unitsampexp2}
    \end{align}

\subsection{Expectation of HT estimator for population mean}   
  For any treatment $t$,
   \begin{align}
   	\E( \hat \mu_{t,\text{HT,SRS}}) &= \E\left(\ell \sum_{c=1}^{\ell} \frac{S_cT_{ct}}{\#T_t}
		\frac{n_c}{n}\sum_{k=1}^{n_c} \frac{y_{kct}S_{kc}}{s_c}\right) 
		\nn&= \ell \sum_{c=1}^{\ell}\frac{n_c}{n}\sum_{k=1}^{n_c} \frac{y_{kct}}{s_c}\E\left(\frac{S_cT_{ct}S_{kc}}{\#T_t}\right) 
		\nn&= \ell \sum_{c=1}^{\ell}\frac{n_c}{n}\sum_{k=1}^{n_c} \frac{y_{kct}}{s_c}\E\left(\E\left(\left.\frac{S_cT_{ct}S_{kc}}{\#T_t} \right|\mathbf{S}\right)\right) 
		\nn&= \ell \sum_{c=1}^{\ell}\frac{n_c}{n}\sum_{k=1}^{n_c} \frac{y_{kct}}{s_c}\E\left(S_c\E\left(\left.\frac{T_{ct}}{\#T_t} \right| \mathbf S \right)\E\left(S_{kc}| \mathbf{S}\right)\right)
		\nn &= \frac{\ell}{s} \sum_{c=1}^{\ell} \frac{1}{n}\sum_{k=1}^{n_c} y_{kct} \E(S_c)
		\nn &= \sum_{c=1}^{\ell}\sum_{k=1}^{n_c} \frac{y_{kct}}{n}  = \mu_t. \label{htexpmu}
  \end{align}

\subsection{Variance of HT estimator for population mean}  

By the law of total variance,
\begin{align}
    \var(\hat\mu_{t,\text{HT},\text{SRS}}) ={}& \var \left[ \E\left(\left. \ell\sum_{c=1}^\ell \frac{S_c T_{ct}}{\#T_t}\frac{n_c}{n} \sum_{k=1}^{n_c}\frac{y_{kct}S_{kc}}{s_c} \right| \mathbf{S}, \mathbf{T} \right) \right] 
    \nn {}& + \E\left[ \var\left(\left. \ell\sum_{c=1}^\ell \frac{S_c T_{ct}}{\#T_t}\frac{n_c}{n} \sum_{k=1}^{n_c}\frac{y_{kct}S_{kc}}{s_c} \right| \mathbf{S}, \mathbf{T} \right) \right].
\end{align}
\noindent
Let's focus on deriving and simplifying each term separately.  The first term:
\begin{align}
  {}&\var \left[ \E\left(\left. \ell\sum_{c=1}^\ell \frac{S_c T_{ct}}{\#T_t}\frac{n_c}{n} \sum_{k=1}^{n_c}\frac{y_{kct}S_{kc}}{s_c} \right| \mathbf{S}, \mathbf{T} \right) \right] = \var\left[ \ell\sum_{c=1}^\ell \frac{S_cT_{ct}}{\#T_t}\frac{n_c}{n} \E\left(\left.\sum_{k=1}^{n_c}\frac{y_{kct}S_{kc}}{s_c} \right| \mathbf{S}, \mathbf{T} \right)\right]
  \nn {}&= \var\left[\ell \sum_{c=1}^\ell \frac{S_cT_{ct}}{\#T_t}\frac{n_c}{n}\mu_{ct}\right]
  \nn {}& = \ell^2 \sum_{c=1}^\ell \sum_{c'=1}^\ell \frac{n_c n_{c'}}{n^2}\mu_{ct}\mu_{c't}\cov\left[\frac{S_cT_{ct}}{\#T_t},  \frac{S_{c'}T_{c't}}{\#T_t}\right]
  \nn {}& = \ell^2 \sum_{c=1}^\ell \frac{n_c^2}{n^2}\mu_{ct}^2\var\left[\frac{S_cT_{ct}}{\#T_t}\right] + \ell \sum_{c=1}^\ell \sum_{c'\neq c} \frac{n_c n_{c'}}{n^2}\mu_{ct}\mu_{c't}\cov\left[\frac{S_cT_{ct}}{\#T_t},  \frac{S_{c'}T_{c't}}{\#T_t}\right]
  \nn {}& = \E\left(\frac{1}{\#T_t}\right) \ell\sum_{c=1}^\ell \frac{n_c^2}{n^2}\mu_{ct}^2  + \E\left(1-\frac{1}{\#T_t}\right)\frac{\ell}{\ell-1} \sum_{c=1}^\ell \sum_{c'\neq c} \frac{n_cn_{c'}}{n^2}\mu_{ct}\mu_{c't} 
  \nn {}& \hspace{3ex} - \sum_{c=1}^\ell \frac{n_c^2}{n^2}\mu_{ct}^2 - \sum_{c=1}^\ell \sum_{c \neq c} \frac{n_cn_{c'}}{n^2} \mu_{ct}\mu_{c't}
  \nn {}& = \E\left(\frac{1}{\#T_t}\right) \ell\sum_{c=1}^\ell \frac{n_c^2}{n^2}\mu_{ct}^2  + \E\left(1-\frac{1}{\#T_t}\right)\frac{\ell}{\ell-1} \sum_{c=1}^\ell \sum_{c'\neq c} \frac{n_cn_{c'}}{n^2}\mu_{ct}\mu_{c't}  - \mu_t^2 
  \nn {}& =  \E\left(\frac{1}{\#T_t}\right) \ell\sum_{c=1}^\ell \frac{n_c^2}{n^2}\mu_{ct}^2  - \E\left(\frac{1}{\#T_t}\right)  \mu_t^2 
  \nn {}& \hspace{3ex} + \E\left(1-\frac{1}{\#T_t}\right)\frac{\ell}{\ell-1} \sum_{c=1}^\ell \sum_{c'\neq c} \frac{n_cn_{c'}}{n^2}\mu_{ct}\mu_{c't}  - \E\left(1-\frac{1}{\#T_t}\right) \mu_t^2
  \nn {}& = \E\left(\frac{1}{\#T_t}\right) \left[\ell \sum_{c=1}^\ell \frac{n_c^2}{n^2} \mu_{ct}^2 - \mu_t^2\right] + \E\left(\frac{1}{\#T_t}\right) \left[\frac{\ell}{\ell-1}\sum_{c=1}^\ell \sum_{c'\neq c} \frac{n_cn_{c'}}{n^2} \mu_{ct}\mu_{c't} - \mu_t^2 \right] 
  \nn {}& = \E\left(\frac{1}{\#T_t}\right) \left[\ell\sum_{c=1}^\ell \frac{n_c^2}{n^2}\mu_{ct}^2 - \left(\sum_{c=1}^\ell \frac{n_c}{n}\mu_{ct}\right)^2 \right] 
  \nn {}& \hspace{3ex} + \E\left(1-\frac{1}{\#T_t}\right)\left[\frac{\ell}{\ell-1}\sum_{c=1}^\ell \sum_{c'=1}^\ell\frac{n_cn_{c'}}{n^2}\mu_{ct}\mu_{c't} - \frac{\ell}{\ell-1} \sum_{c=1}^\ell \frac{n_c^2}{n^2}\mu_{ct}^2 - \mu_t^2 \right] 
  \nn {}& = \E\left(\frac{1}{\#T_t}\right) \left[\ell\sum_{c=1}^\ell \frac{n_c^2}{n^2}\mu_{ct}^2 - \ell^2\left(\frac{1}{\ell}\sum_{c=1}^\ell \frac{n_c}{n}\mu_{ct}\right)^2 \right]  + \E\left(1-\frac{1}{\#T_t}\right)\left[\frac{1}{\ell-1}\mu_t^2 - \frac{\ell}{\ell-1} \sum_{c=1}^\ell \frac{n_c^2}{n^2}\mu_{ct}^2 \right] 
  \nn {}& = \E\left(\frac{1}{\#T_t}\right)\ell(\ell-1) \left[\frac{1}{\ell-1}\sum_{c=1}^\ell \frac{n_c^2}{n^2}\mu_{ct}^2 - \frac{\ell}{\ell-1}\left(\frac{1}{\ell}\sum_{c=1}^\ell \frac{n_c}{n}\mu_{ct}\right)^2 \right]  
  \nn {}& \hspace{3ex} - \E\left(1-\frac{1}{\#T_t}\right)\frac{1}{\ell-1}\left[\ell\sum_{c=1}^\ell \frac{n_c^2}{n^2}\mu_{ct}^2-\mu_t^2 \right] 
  \nn {}& = \E\left(\frac{1}{\#T_t}\right) \ell(\ell-1)\var\left(\frac{n_c}{n}\mu_{ct}\right) - \E\left(1-\frac{1}{\#T_t}\right)\ell\var\left(\frac{n_c}{n}\mu_{ct}\right)
  \nn {}& = \ell\var\left(\frac{n_c}{n}\mu_{ct}\right) \left[\E\left(\frac{1}{\#T_t}\right)(\ell-1) - \E\left(1-\frac{1}{\#T_t}\right)\right]
  \nn {}& = \ell^2 \left[\E\left(\frac{1}{\#T_t}\right)-\frac{1}{\ell} \right]\var\left(\frac{n_c}{n}\mu_{ct}\right).
\end{align}
\noindent
Since units are sampled independently across clusters, the second term is:
\begin{align}
  {}& \E\left[ \var\left(\left. \ell\sum_{c=1}^\ell \frac{S_c T_{ct}}{\#T_t}\frac{n_c}{n} \sum_{k=1}^{n_c}\frac{y_{kct}S_{kc}}{s_c} \right| \mathbf{S}, \mathbf{T} \right) \right] = \E\left[\ell^2 \sum_{c=1}^\ell \frac{S_c^2T_{ct}^2}{\#T_t^2}\frac{n_c^2}{n^2}\var\left(\left.\hat\mu_{ct}\right|\mathbf{S}, \mathbf{T} \right) \right]
  \nn {}&  = \E\left[\ell^2 \sum_{c=1}^\ell \frac{S_c^2T_{ct}^2}{\#T_t^2} \frac{n_c^2}{n^2}\var(\hat\mu_{ct}|\mathbf{S}, \mathbf{T})\right]
    \nn  {}&  = \ell^2 \sum_{c=1}^\ell \frac{n_c^2}{n^2}\var(\hat\mu_{ct}|\mathbf{S}, \mathbf{T})\E\left[\frac{S_c^2T_{ct}^2}{\#T_t^2}\right]
    \nn {}& = \E\left(\frac{1}{\#T_t}\right) \ell \sum_{c=1}^\ell \frac{n_c^2}{n^2} \var(\hat\mu_{ct})
    \nn {}&  = \E\left(\frac{1}{\#T_t}\right) \ell \sum_{c=1}^\ell \frac{n_c^2}{n^2} \left[ \var\left( \sum_{k=1}^{n_c} \frac{y_{kct}S_{kc}}{s_c} \right)  + \cov\left( \sum_{k=1}^{n_c} \frac{y_{kct}S_{kc}}{s_c}, \sum_{k'\neq k} \frac{y_{k'ct}S_{k'c}}{s_c} \right) \right]
    \nn {}& = \E\left(\frac{1}{\#T_t}\right) \ell \sum_{c=1}^\ell \frac{n_c^2}{n^2} \left[ \sum_{k=1}^{n_c} \frac{y_{kct}^2}{s_c^2} \frac{s_c}{n_c}\left(1-\frac{s_c}{n_c} \right) - \sum_{k=1}^{n_c}\sum_{k'\neq k}\frac{y_{kct}y_{k'ct}}{s_c^2}\frac{s_c}{n_c(n_c-1)}\left(1-\frac{s_c}{n_c}\right) \right]
   \nn {}& = \E\left(\frac{1}{\#T_t}\right) \ell \sum_{c=1}^\ell \frac{n_c}{n^2s_c}\left(1-\frac{s_c}{n_c}\right)\frac{1}{(n_c-1)}\left[ (n_c-1)\sum_{k=1}^{n_c} y_{kct}^2-\sum_{k=1}^{n_c}\sum_{k'\neq k}y_{kct}y_{k'ct} \right]
   \nn {}& = \E\left(\frac{1}{\#T_t}\right) \ell \sum_{c=1}^\ell \frac{n_c}{n^2s_c}\left(1-\frac{s_c}{n_c}\right)\frac{1}{(n_c-1)}\left[ (n_c-1)\sum_{k=1}^{n_c}y_{kct}^2-\sum_{k=1}^{n_c}\sum_{k'=1}^{n_c}y_{kct}y_{k'ct} + \sum_{k=1}^{n_c}y_{kct}^2 \right]
   \nn {}& = \E\left(\frac{1}{\#T_t}\right) \ell \sum_{c=1}^\ell \frac{n_c}{n^2s_c}\left(1-\frac{s_c}{n_c}\right)\frac{1}{(n_c-1)} \left[ n_c\sum_{k=1}^{n_c}y_{kct}^2-\left(\sum_{k=1}^{n_c}y_{kct}\right)^2 \right]  
   \nn {}& = \E\left(\frac{1}{\#T_t}\right) \ell \sum_{c=1}^\ell \frac{n_c^2}{n^2}\left(1-\frac{s_c}{n_c}\right)\frac{\var(y_{kct})}{s_c}.   
\end{align}
\noindent
Thus, the variance of the HT estimator for $\mu_t$ is
\begin{equation}
  \var(\hat\mu_{t,\text{HT},\text{SRS}}) = \ell^2 \left[\E\left(\frac{1}{\#T_t}\right)-\frac{1}{\ell} \right]\var\left(\frac{n_c}{n}\mu_{ct}\right) + \E\left(\frac{1}{\#T_t}\right) \ell \sum_{c=1}^\ell \frac{n_c^2}{n^2}\left(1-\frac{s_c}{n_c}\right)\frac{\var(y_{kct})}{s_c}
    \label{htvarmu}
\end{equation}
where $\var\left(\frac{n_c}{n}\mu_{ct}\right)$ is the population variance of weighted cluster means and $\var(y_{kct})$ is the population variance of outcomes in a cluster.

\subsection{Covariance of HT estimator for the population means}

We derive the covariance term through the property:
\begin{equation}
\cov(\hat{\mu}_{1,\text{HT, SRS}}) = \E(\hat{\mu}_{1,\text{HT, SRS}} \hat{\mu}_{0,\text{HT, SRS}} ) - \E(\hat{\mu}_{1,\text{HT, SRS}}) \E(\hat{\mu}_{0,\text{HT, SRS}}).
\end{equation}  
\noindent
Note that:
\begin{align}
\hat{\mu}_{1,\text{HT, SRS}} \hat{\mu}_{0,\text{HT, SRS}} &= \left( \ell \sum\limits_{c=1}^{\ell} \frac{S_c T_{c1}}{\#T_1} \frac{n_c}{n} \sum\limits_{k=1}^{n_c} \frac{y_{kc1}S_{kc}}{s_c} \right) \left(  \ell \sum\limits_{c'=1}^{\ell} \frac{S_{c'}T_{c'0}}{\#T_0} \frac{n_{c'}}{n} \sum\limits_{k^*=1}^{n_{c'}} \frac{y_{k^*c'0}S_{k^*c'}}{s_{c'}} \right)
\nn &= \ell^2 \sum\limits_{c=1}^\ell \sum\limits_{k=1}^{n_c} \sum\limits_{c'=1}^\ell \sum\limits_{k^*=1}^{n_{c'}} \frac{n_cn_{c'}}{n^2}\frac{y_{kc1} y_{k^*c'0}}{s_c s_{c'}} \frac{S_c S_{c'} T_{c1} T_{c'0} S_{kc} S_{k^*c'}}{\#T_1\#T_0}
\nn &= \ell^2 \sum\limits_{c=1}^\ell \sum\limits_{k=1}^{n_c} \sum\limits_{c'\neq c} \sum\limits_{k^*=1}^{n_{c'}} \frac{n_cn_{c'}}{n^2}\frac{y_{kc1} y_{k^*c'0}}{s_c s_{c'}} \frac{S_c S_{c'} T_{c1} T_{c'0} S_{kc} S_{k^*c'}}{\#T_1\#T_0}.
\end{align}
\noindent
The last equality comes from the fact that a cluster can only be given one treatment.  Then:
\begin{align}
\E(\hat{\mu}_{1,\text{HT, SRS}} \hat{\mu}_{0,\text{HT, SRS}}) &= \E \left( \ell^2 \sum\limits_{c=1}^\ell \sum\limits_{k=1}^{n_c} \sum\limits_{c'\neq c} \sum\limits_{k^*=1}^{n_{c'}} \frac{n_cn_{c'}}{n^2}\frac{y_{kc1} y_{k^*c'0}}{s_c s_{c'}} \frac{S_c S_{c'} T_{c1} T_{c'0} S_{kc} S_{k^*c'}}{\#T_1\#T_0} \right)
\nn &=  \ell^2  \sum\limits_{c=1}^\ell \sum\limits_{k=1}^{n_c} \sum\limits_{c'\neq c} \sum\limits_{k^*=1}^{n_{c'}} \frac{n_cn_{c'}}{n^2}  \frac{y_{kc1} y_{k^*c'0}}{s_c s_{c'}} \E \left( \frac{S_c S_{c'} T_{c1} T_{c'0} S_{kc} S_{k^*c'}}{\#T_1\#T_0} \right)
\nn &=  \ell^2 \sum\limits_{c=1}^\ell \sum\limits_{k=1}^{n_c} \sum\limits_{c'\neq c} \sum\limits_{k^*=1}^{n_{c'}} \frac{n_cn_{c'}}{n^2} \frac{y_{kc1} y_{k^*c'0}}{s_c s_{c'}} \E \left( \frac{S_c S_{c'}T_{c1} T_{c'0}}{\#T_1\#T_0} \E(S_{kc} S_{k^*c'}|\mathbf{S, T}) \right)
\nn &=  \ell^2 \sum\limits_{c=1}^\ell \sum\limits_{c'\neq c}  \frac{n_cn_{c'}}{n^2} \mu_{c1}\mu_{c'0} \E\left(\frac{1}{\#T_1\#T_0} \E\left( S_c S_{c'}T_{c1} T_{c'0} |\#T_1, \#T_0 \right)\right)
\nn &= \frac{\ell}{\ell-1} \sum\limits_{c=1}^\ell \sum\limits_{c\neq c'} \frac{n_cn_{c'}}{n^2} \mu_{c1} \mu_{c'0}.
\end{align}

Therefore:
\begin{equation}
\cov(\hat{\mu}_{1,\text{HT, SRS}}) = \frac{\ell}{\ell-1} \sum\limits_{c=1}^\ell \sum\limits_{c\neq c'} \frac{n_cn_{c'}}{n^2} \mu_{c1} \mu_{c'0} - \mu_1\mu_0.
\label{dericovHT}
\end{equation} 

\subsection{Linear transforms on HT estimator for the population mean}
Observe that, for any constants $a, b$:
\begin{align}
	\hat \mu_{t,\text{HT,SRS}}(a + b \mathbf y)  &=
		\ell\sum_{c=1}^{\ell} \frac{S_cT_{ct}}{\#T_t}\frac{n_c}{n}\sum_{k=1}^{n_c} \frac{(a+by_{kct})S_{kc}}{s_c} 
		\nn &= \ell\sum_{c=1}^{\ell} \frac{S_cT_{ct}}{\#T_t}\frac{n_c}{n}\sum_{k=1}^{n_c} \frac{aS_{kc}}{s_c} + \ell\sum_{c=1}^{\ell} \frac{S_cT_{ct}}{\#T_t}\frac{n_c}{n}\sum_{k=1}^{n_c} \frac{by_{kct}S_{kc}}{s_c}
		\nn &= a \ell\sum_{c=1}^{\ell} \frac{S_cT_{ct}}{\#T_t}\frac{n_c}{n}\sum_{k=1}^{n_c} \frac{S_{kc}}{s_c} + b\ell\sum_{c=1}^{\ell} \frac{S_cT_{ct}}{\#T_t}\frac{n_c}{n}\sum_{k=1}^{n_c} \frac{y_{kct}S_{kc}}{s_c}
		\nn &= a \ell\sum_{c=1}^{\ell} \frac{S_cT_{ct}}{\#T_t}\frac{n_c}{n} + b\hat \mu_{t,\text{HT,SRS}}(\mathbf{y})
		\nn&=
		a \frac{\ell\#N_t}{n\#T_t} + b\hat \mu_{t,\text{HT,SRS}}(\mathbf{y}). \label{htlinearmu}
\end{align}

\subsection{Proof of lemma~\ref{HTSRSlemma}} \label{htsrslemmaproof}

Equation~\eqref{htexpmu} shows that $\hat\mu_{t,\text{HT,SRS}}$ is unbiased for $\mu_t$ since
\begin{align}
  \E(\left(\hat{\delta}_{\text{HT,SRS}} \right) &= \E(\hat\mu_{1,\text{HT,SRS}}) - \E(\hat\mu_{0,\text{HT,SRS}})
  \nn &= \mu_1-\mu_0 
  \nn &= \delta. 
\end{align}
\noindent
From~\eqref{htvarmu} and~\eqref{dericovHT}, the variance of the Horvitz-Thompson estimator of PATE is
\begin{align}
  \var\left(\hat{\delta}_{\text{HT,SRS}} \right) ={}& \var\left(\hat\mu_{1,\text{HT,SRS}}\right)+\var\left(\hat\mu_{0,\text{HT,SRS}}\right) - 2\cov(\hat\mu_{1,\text{HT,SRS}}, \hat\mu_{0,\text{HT,SRS}})
  \nn ={}& \ell^2 \left[\E\left(\frac{1}{\#T_1}\right)-\frac{1}{\ell} \right]\var\left(\frac{n_c}{n}\mu_{c1}\right) + \E\left(\frac{1}{\#T_1}\right) \ell \sum_{c=1}^\ell \frac{n_c^2}{n^2}\left(1-\frac{s_c}{n_c}\right)\frac{\var(y_{kc1})}{s_c}
  \nn {}& + \ell^2 \left[\E\left(\frac{1}{\#T_0}\right)-\frac{1}{\ell} \right]\var\left(\frac{n_c}{n}\mu_{c0}\right) + \E\left(\frac{1}{\#T_0}\right) \ell \sum_{c=1}^\ell \frac{n_c^2}{n^2}\left(1-\frac{s_c}{n_c}\right)\frac{\var(y_{kc0})}{s_c}
     \nn {}& + 2 \frac{\ell}{\ell-1} \sum\limits_{c=1}^\ell \sum\limits_{c\neq c'} \frac{n_cn_{c'}}{n^2} \mu_{c1} \mu_{c'0} - 2\mu_1\mu_0.
\end{align}
\noindent
Finally, from~\ref{htlinearmu}, the PATE for linearly transformed outcomes is 
\begin{align}
  \hat\delta_{\text{HT,SRS}}(a+\mathbf{y}) &= \hat \mu_{1,\text{HT,SRS}}(a + \mathbf y) - \hat \mu_{0,\text{HT,SRS}}(a + \mathbf y)
  \nn &=  \left(a \frac{\ell\#N_1}{n\#T_1}	+ \hat \mu_{1,\text{HT,SRS}}(\mathbf{y})\right) - \left(a \frac{\ell\#N_0}{n\#T_0} + b\hat \mu_{0,\text{HT,SRS}}(\mathbf{y}) \right)
  \nn &= a\frac{\ell}{n}\left( \frac{\#N_1}{\#T_1}-\frac{\#N_0}{\#T_0} \right) + \hat\delta_{\text{HT,SRS}}(\mathbf{y}).
\end{align}

\subsection{Variance of PATE estimator for transformed outcomes}

For linearly transformed potential outcomes, the variance will then be
\begin{align}
  \var(\hat{\delta}_{\text{HT,SRS}}(a+\mathbf{y})) ={}& \var\left[ a\frac{\ell}{n} \left( \frac{\#N_1}{\#T_1} - \frac{\#N_0}{\#T_0} \right) + \hat{\delta}_{\text{HT,SRS}} \right]
    \nn ={}& \var\left[ a\frac{\ell}{n} \left( \frac{\#N_1}{\#T_1} - \frac{\#N_0}{\#T_0} \right) \right] + \var\left( \hat{\delta}_{\text{HT,SRS}} \right) 
    \nn {}&  + 2 \cov\left[ a\frac{\ell}{n} \left( \frac{\#N_1}{\#T_1}-\frac{\#N_0}{\#T_0} \right), \hat{\delta}_{\text{HT,SRS}} \right]
    \nn ={}& a^2 \left(\frac{\ell}{n}\right)^2 \var\left(\frac{\#N_1}{\#T_1}-\frac{\#N_0}{\#T_0}\right) + 2a\frac{\ell}{n} \cov\left(\frac{\#N_1}{\#T_1}-\frac{\#N_0}{\#T_0}, \hat{\delta}_{\text{HT,SRS}}\right) 
    \nn {}& + \var(\hat{\delta}_{\text{HT,SRS}})
    \nn ={}& a^2 \left(\frac{\ell}{n}\right)^2 \left[\var\left(\frac{\#N_1}{\#T_1}\right) + \var\left(\frac{\#N_0}{\#T_0}\right)-2\cov\left(\frac{\#N_1}{\#T_1}, \frac{\#N_0}{\#T_0}\right)\right] 
    \nn {}& + 2a\frac{\ell}{n} \left[ \cov\left(\frac{\#N_1}{\#T_1}, \hat{\delta}_{\text{HT,SRS}}\right) - \cov\left(\frac{\#N_0}{\#T_0}, \hat{\delta}_{\text{HT,SRS}}\right) \right] 
    \nn {}& + \var(\hat{\delta}_{\text{HT,SRS}}).
\end{align}
