# Supplementary material for: The Benefits of Probability-Proportional-to-Size Sampling in Cluster-Randomized Experiments
Source: arXiv:2002.08009 source file (2020-02-19)
Supplement: Supplementary file 2 [file AppendixB-dim.tex]

\cleardoublepage

\section{Properties of the DIM estimator} \label{appendixdim}

We begin by investigating the properties of $\hat\mu_{t,\text{DIM,SRS}}$.  Then using these properties, we prove lemma~\ref{dimlemma}.  

\subsection{Expectation of DIM estimator for population mean} 

Since the DIM estimator of $\mu_t$ is a ratio estimator, following \citet{lohr2010sampling} and \citet{middleton2015unbiased}, we can use the following relationship to calculate the expectation of the DIM estimator.  When both $u$ and $v \geq 0$ are random, it can be shown that
  \begin{align}
  \E\left(\frac{u}{v}\right) = \frac{1}{\E(v)} \left[\E(u)-\cov\left(\frac{u}{v},v\right) \right] \label{ratioest}.
  \end{align}
Given that,

\begin{align}
    \E\left(\sum_{c=1}^\ell S_cT_{ct}\sum_{k=1}^{n_c}y_{kct}S_{kc}\right) &= \sum_{c=1}^\ell \sum_{k=1}^{n_c} \frac{\#T_t}{\ell}\frac{s_c}{n_c} y_{kct} \\
    \E\left(\sum_{c=1}^\ell S_cT_{ct}s_c\right) &= \sum_{c=1}^\ell \frac{\#T_t}{\ell}s_c,
\end{align}
the expectation of the DIM estimator for the population mean is
\begin{align}
    \E(\hat\mu_{t,\text{DIM, SRS}}) &= \E\left( \frac{\sum_{c=1}^\ell S_cT_{ct}\sum_{k=1}^{n_c}y_{kct}S_{kc}}{\sum_{c=1}^\ell S_cT_{ct}s_c} \right) 
    \nn &= \frac{1}{\sum_{c=1}^\ell s_c}\left[ \sum_{c=1}^\ell \sum_{k=1}^{n_c} \frac{s_c}{n_c} y_{kct} - \frac{\ell}{\#T_t}\cov\left( \hat\mu_{t,\text{DIM, SRS}}, \sum_{c=1}^\ell S_cT_{ct}s_c 
    \right)\right] \label{dimexpmu}
\end{align}

\subsection{Variance of DIM estimator for population mean} 

Let
\begin{align}
    \hat\tau^*_{ct} &= \sum_{k=1}^{n_c}y_{kct}S_{kc},\\
    \tau^*_{ct} &= \sum_{k=1}^{n_c} \frac{s_c}{n_c} y_{kct}
\end{align}
and
\begin{equation}
        \mu^*_{t, \text{DIM}} = \frac{\sum_{c=1}^\ell \sum_{k=1}^{n_c} \frac{s_c}{n_c} y_{kct}}{\sum_{c=1}^\ell s_c}. 
\end{equation}
Using Taylor series expansion, the DIM estimator can be approximated by
\begin{equation}
    \hat\mu_{t, \text{DIM, SRS}} \approx \mu^*_{t, \text{DIM}} + \frac{\ell}{\sum_{c=1}^\ell s_c} \sum_{c=1}^\ell \frac{S_cT_{ct}}{\#T_t}\left( \hat\tau^*_{ct}-\mu^*_{t, \text{DIM}}s_c \right). \label{dimtaylorexp}
\end{equation}
Then
\begin{align}
   &{}\var(\hat\mu_{t,\text{DIM, SRS}}) 
   \nn &{} \approx \frac{1}{\left(\sum_{c=1}^\ell s_c\right)^2}\sum_{c=1}^\ell \sum_{c'=1}^\ell \ell^2 \cov\left[ \frac{S_cT_{ct}}{\#T_t}\left( \hat\tau^*_{ct} - \mu^*_{t, \text{DIM}}s_c \right), \frac{S_{c'}T_{c't}}{\#T_t}\left( \hat\tau^*_{c't} - \mu^*_{t, \text{DIM}}s_{c'} \right) \right]
    \nn &{} = \frac{1}{\left(\sum_{c=1}^\ell s_c\right)^2}\sum_{c=1}^\ell \sum_{c'=1}^\ell \ell^2 \cov\bigg( \E\bigg[ \frac{S_cT_{ct}}{\#T_t} \left. \left( \hat\tau^*_{ct}-\mu^*_{t, \text{DIM}}s_c \right) \right| \mathbf{S, T} \bigg], \E\bigg[ \frac{S_{c'}T_{c't}}{\#T_t} \left. \left(  \hat\tau^*_{c't}-\mu^*_{t, \text{DIM}}s_{c'} \right) \right| \mathbf{S, T} \bigg]  \bigg) 
    \nn &{} \qquad + \frac{1}{\left(\sum_{c=1}^\ell s_c\right)^2}\sum_{c=1}^\ell \sum_{c'=1}^\ell \ell^2 \E\left(  \cov\bigg[ \frac{S_cT_{ct}}{\#T_t}\left( \hat\tau^*_{ct} - \mu^*_{t, \text{DIM}}s_c\right), \frac{S_{c'}T_{c't}}{\#T_t} \bigg. \left( \hat\tau^*_{c't}-\mu^*_{t, \text{DIM}}s_{c'} \right) \bigg| \mathbf{S, T} \bigg] \right) \label{dimvarlaw}.
\end{align}   
Focusing on the first term of \eqref{dimvarlaw}:
\begin{align}
    {}&\sum_{c=1}^\ell \sum_{c'=1}^\ell \ell^2 \cov\bigg( \E\bigg[ \frac{S_cT_{ct}}{\#T_t} \left. \left( \hat\tau^*_{ct}-\mu^*_{t, \text{DIM}}s_c \right) \right| \mathbf{S, T} \bigg], \E\bigg[ \frac{S_{c'}T_{c't}}{\#T_t} \left. \left(  \hat\tau^*_{c't}-\mu^*_{t, \text{DIM}}s_{c'} \right) \right| \mathbf{S, T} \bigg]  \bigg)
    \nn {}& = \sum_{c=1}^\ell \sum_{c'=1}^\ell \ell^2 \cov\bigg[ \frac{S_cT_{ct}}{\#T_t} \left( \tau^*_{ct}-\mu^*_{t, \text{DIM}}s_c \right), \frac{S_{c'}T_{c't}}{\#T_t}\left(  \tau^*_{c't}-\mu^*_{t, \text{DIM}}s_{c'} \right) \bigg]
    \nn {}& = \sum_{c=1}^\ell \sum_{c'=1}^\ell \ell^2 \left( \tau^*_{ct}-\mu^*_{t, \text{DIM}}s_c \right)\left(  \tau^*_{c't}-\mu^*_{t, \text{DIM}}s_{c'} \right) \cov\left(  \frac{S_cT_{ct}}{\#T_t}, \frac{S_{c'}T_{c't}}{\#T_t}\right)    
    \nn {}& = \sum_{c=1}^\ell \ell^2 \left( \tau^*_{ct}-\mu^*_{t, \text{DIM}}s_c \right)^2\var\left(\frac{S_cT_{ct}}{\#T_t}\right) 
    \nn {}& \qquad + \sum_{c=1}^\ell \sum_{c'\neq c} \ell^2 \left( \tau^*_{ct}-\mu^*_{t, \text{DIM}}s_c \right)\left(  \tau^*_{c't}-\mu^*_{t, \text{DIM}}s_{c'} \right) \cov\left(  \frac{S_cT_{ct}}{\#T_t}, \frac{S_{c'}T_{c't}}{\#T_t}\right) 
    \nn {}& = \sum_{c=1}^\ell \left[\E\left(\frac{1}{\#T_t}\right)\ell -1\right] \left( \tau^*_{ct}-\mu^*_{t, \text{DIM}}s_c \right)^2
    \nn {}& \qquad - \sum_{c=1}^\ell \sum_{c'\neq c} \left[\E\left(1-\frac{1}{\#T_t}\right) \frac{\ell}{(\ell-1)}-1\right] \left( \tau^*_{ct}-\mu^*_{t, \text{DIM}}s_c \right)\left(  \tau^*_{c't}-\mu^*_{t, \text{DIM}}s_{c'} \right)  
    \nn {}& = \E\left(\frac{1}{\#T_t}\right)\ell \sum_{c=1}^\ell \left(\tau^*_{ct}-\mu^*_{t,\text{DIM}}s_c\right)^2 - \sum_{c=1}^\ell \left(\tau^*_{ct}-\mu^*_{t,\text{DIM}}s_c\right)^2
    \nn {}& \hspace{3ex} + \E\left(1-\frac{1}{\#T_t}\right)\frac{\ell}{\ell-1} \sum_{c=1}^\ell \sum_{c'\neq c}   \left(\tau^*_{ct}-\mu^*_{t,\text{DIM}}s_c\right) \left(\tau^*_{c't}-\mu^*_{t,\text{DIM}}s_{c'}\right) 
    \nn {}& \hspace{3ex} - \sum_{c=1}^\ell \sum_{c'\neq c} \left(\tau^*_{ct}-\mu^*_{t,\text{DIM}}s_c\right) \left(\tau^*_{c't}-\mu^*_{t,\text{DIM}}s_{c'}\right)
    \nn {}& = \E\left(\frac{1}{\#T_t}\right)\ell \sum_{c=1}^\ell \left(\tau^*_{ct}-\mu^*_{t,\text{DIM}}s_c\right)^2 
    \nn {}& \hspace{3ex} + \E\left(1-\frac{1}{\#T_t}\right)\frac{\ell}{\ell-1} \sum_{c=1}^\ell \sum_{c'\neq c}   \left(\tau^*_{ct}-\mu^*_{t,\text{DIM}}s_c\right) \left(\tau^*_{c't}-\mu^*_{t,\text{DIM}}s_{c'}\right) 
    \nn {}& \hspace{3ex} - \ell^2 \left[ \frac{1}{\ell}\sum_{c=1}^\ell  \left(\tau^*_{ct}-\mu^*_{t,\text{DIM}}s_c\right)\right]^2
    \nn {}& = \E\left(\frac{1}{\#T_t}\right)\left(\ell \sum_{c=1}^\ell \left(\tau^*_{ct}-\mu^*_{t,\text{DIM}}s_c\right)^2 - \ell^2 \left[ \frac{1}{\ell}\sum_{c=1}^\ell  \left(\tau^*_{ct}-\mu^*_{t,\text{DIM}}s_c\right)\right]^2\right)
    \nn {}& \hspace{3ex} + \E\left(1-\frac{1}{\#T_t}\right) \left(\frac{\ell}{\ell-1} \sum_{c=1}^\ell \sum_{c'\neq c}   \left(\tau^*_{ct}-\mu^*_{t,\text{DIM}}s_c\right) \left(\tau^*_{c't}-\mu^*_{t,\text{DIM}}s_{c'}\right) \right.
    \nn {}& \hspace{50ex} \left. - \ell^2 \left[ \frac{1}{\ell}\sum_{c=1}^\ell  \left(\tau^*_{ct}-\mu^*_{t,\text{DIM}}s_c\right)\right]^2\right)
    \nn {}& = \E\left(\frac{1}{\#T_t}\right) \ell(\ell-1)\left(\frac{1}{\ell-1} \sum_{c=1}^\ell \left(\tau^*_{ct}-\mu^*_{t,\text{DIM}}s_c\right)^2 - \frac{\ell}{\ell-1} \left[ \frac{1}{\ell}\sum_{c=1}^\ell  \left(\tau^*_{ct}-\mu^*_{t,\text{DIM}}s_c\right)\right]^2\right)
    \nn {}& \hspace{3ex} + \E\left(1-\frac{1}{\#T_t}\right) \left(\frac{\ell}{\ell-1} \sum_{c=1}^\ell \sum_{c'=1}^\ell   \left(\tau^*_{ct}-\mu^*_{t,\text{DIM}}s_c\right) \left(\tau^*_{c't}-\mu^*_{t,\text{DIM}}s_{c'}\right) \right.
    \nn {}& \hspace{23ex} \left. - \frac{\ell}{\ell-1} \sum_{c=1}^\ell \left(\tau^*_{ct}-\mu^*_{t,\text{DIM}}s_c\right)^2- \ell^2 \left[ \frac{1}{\ell}\sum_{c=1}^\ell  \left(\tau^*_{ct}-\mu^*_{t,\text{DIM}}s_c\right)\right]^2\right)
    \nn {}& =\E\left(\frac{1}{\#T_t}\right) \ell(\ell-1) \var\left[\left(\tau^*_{ct}-\mu^*_{t,\text{DIM}}s_c\right)\right] 
    \nn {}& \hspace{3ex} - \E\left(1-\frac{1}{\#T_t}\right) \ell \left(\frac{1}{\ell-1} \sum_{c=1}^\ell \left(\tau^*_{ct}-\mu^*_{t,\text{DIM}}s_c\right)^2 - \frac{\ell}{\ell-1} \left[ \frac{1}{\ell}\sum_{c=1}^\ell  \left(\tau^*_{ct}-\mu^*_{t,\text{DIM}}s_c\right)\right]^2\right)
    \nn {}& = \ell^2\left[\E\left(\frac{1}{\#T_t}\right) - \frac{1}{\ell}\right] \var\left[\left(\tau^*_{ct}-\mu^*_{t,\text{DIM}}s_c\right)\right]
\end{align}
The second term of \eqref{dimvarlaw}:
\begin{align}
    {}& \ell^2 \sum_{c=1}^\ell \sum_{c'=1}^\ell \E\left( \cov\bigg[ \frac{S_cT_{ct}}{\#T_t}\left( \hat\tau^*_{ct} - \mu^*_{t, \text{DIM}}s_c\right), \frac{S_{c'}T_{c't}}{\#T_t} \bigg. \left( \hat\tau^*_{c't}-\mu^*_{t, \text{DIM}}s_{c'} \right) \bigg| \mathbf{S, T} \bigg] \right)
    \nn {}&= \ell^2 \sum_{c=1}^\ell \sum_{c'=1}^\ell \E\left[  \frac{S_cS_{c'}T_{ct}T_{c't}}{\#T_t^2}  \cov\left( \hat\tau^*_{ct}, \hat\tau^*_{c't}\right) \right]
    \nn {}&= \ell^2 \sum_{c=1}^\ell \var\left( \hat\tau^*_{ct}\right) \E\left(\frac{S_c^2T_{ct}^2}{\#T_t^2}\right) 
    \nn {}&=  \E\left(\frac{1}{\#T_t}\right) \ell \sum_{c=1}^\ell\var\left( \sum_{k=1}^{n_c}y_{kct}S_{kc}\right)    
      \nn {}&= \E\left(\frac{1}{\#T_t}\right) \ell \sum_{c=1}^\ell s_c\left(1-\frac{s_c}{n_c}\right)\var(y_{kct})  
\end{align}
The variance of $\hat\mu_{t,\text{DIM,SRS}}$ is then
\begin{align} %here-change
    \var(\hat\mu_{t,\text{DIM, SRS}}) \approx{}& \frac{\ell^2}{\left(\sum_{c=1}^\ell s_c\right)^2} \left[\E\left(\frac{1}{\#T_t}\right) - \frac{1}{\ell}\right] \var\left[\left(\tau^*_{ct}-\mu^*_{t,\text{DIM}}s_c\right)\right] 
    \nn {}& + \frac{\ell}{\left(\sum_{c=1}^\ell s_c\right)^2} \E\left(\frac{1}{\#T_t}\right) \sum_{c=1}^\ell s_c\left(1-\frac{s_c}{n_c}\right)\var(y_{kct})  \label{dimvarmu}
\end{align}

\subsection{Covariance of DIM estimator for the population means}

Based on the Taylor expansion in eq.~\eqref{dimtaylorexp},
\begin{align}
    {}& \cov(\hat\mu_{1, \text{DIM, SRS}}, \hat\mu_{0, \text{DIM, SRS}}) 
    \nn &\approx  \frac{\ell^2}{\left(\sum_{c=1}^\ell s_c\right)^2}  \cov\left[\sum_{c=1}^\ell \frac{S_cT_{c1}}{\#T_1} \left(\hat\tau^*_{c1}-\mu^*_{1, \text{DIM}}s_c \right), \sum_{c'=1}^\ell \frac{S_{c'}T_{c'0}}{\#T_0}\left(\hat\tau^*_{c'0}-\mu^*_{0, \text{DIM}}s_{c'} \right) \right]
    \nn {}& = \frac{\ell^2}{\left(\sum_{c=1}^\ell s_c\right)^2}  \sum_{c=1}^\ell \sum_{c'=1}^\ell \cov\bigg( \E\bigg[\frac{S_cT_{c1}}{\#T_1} \left.\left(\hat\tau^*_{c1}-\mu^*_{1, \text{DIM}}s_c \right) \right|\mathbf{S, T} \bigg], \E\bigg[\frac{S_{c'}T_{c'0}}{\#T_0}\left.\left(\hat\tau^*_{c'0}-\mu^*_{0, \text{DIM}}s_{c'} \right) \right|\mathbf{S, T} \bigg] \bigg)
    \nn {}& \hspace{3ex} + \frac{\ell^2}{\left(\sum_{c=1}^\ell s_c\right)^2}  \sum_{c=1}^\ell \sum_{c'=1}^\ell \E\bigg(\cov\bigg[\frac{S_cT_{c1}}{\#T_1}\bigg.\left(\hat\tau^*_{c1}-\mu^*_{1, \text{DIM}}s_c \right), \frac{S_{c'}T_{c'0}}{\#T_0}\left(\hat\tau^*_{c'0}-\mu^*_{0, \text{DIM}}s_{c'} \right) \bigg| \mathbf{S, T} \bigg] \bigg)
    \nn {}& = \frac{\ell^2}{\left(\sum_{c=1}^\ell s_c\right)^2} \sum_{c=1}^\ell \sum_{c'=1}^\ell \left(\tau^*_{c1}-\mu^*_{1, \text{DIM}}s_c \right) \left(\tau^*_{c'0}-\mu^*_{0, \text{DIM}}s_{c'} \right) \cov\left( \frac{S_cT_{c1}}{\#T_1}, \frac{S_{c'}T_{c'0}}{\#T_0}\right)
    \nn {}& = \frac{\ell^2}{\left(\sum_{c=1}^\ell s_c\right)^2} \sum_{c=1}^\ell \left(\tau^*_{c1}-\mu^*_{1, \text{DIM}}s_c \right) \left(\tau^*_{c0}-\mu^*_{0, \text{DIM}}s_{c} \right) \var\left( \frac{S_cT_{c1}T_{c0}}{\#T_1\#T_0}\right) 
    \nn {}& \hspace{3ex} \qquad +
    \frac{\ell^2}{\left(\sum_{c=1}^\ell s_c\right)^2} \sum_{c=1}^\ell \sum_{c'\neq c} \left(\tau^*_{c1}-\mu^*_{1, \text{DIM}}s_c \right) \left(\tau^*_{c'0}-\mu^*_{0, \text{DIM}}s_{c'} \right) \cov\left( \frac{S_cT_{c1}}{\#T_1}, \frac{S_{c'}T_{c'0}}{\#T_0}\right)
    \nn {}& = \frac{1}{\left(\sum_{c=1}^\ell s_c\right)^2} \frac{1}{\ell-1} \sum_{c=1}^\ell \sum_{c'\neq c} \left(\tau^*_{c1}-\mu^*_{1, \text{DIM}}s_c \right) \left(\tau^*_{c'0}-\mu^*_{0, \text{DIM}}s_{c'} \right)
    \nn {}& \hspace{3ex} - \frac{1}{\left(\sum_{c=1}^\ell s_c\right)^2} \sum_{c=1}^\ell \left(\tau^*_{c1}-\mu^*_{1, \text{DIM}}s_c \right)\left(\tau^*_{c0}-\mu^*_{0, \text{DIM}}s_c \right)
    \nn {}& = \frac{1}{\left(\sum_{c=1}^\ell s_c\right)^2} \frac{1}{\ell-1} \sum_{c=1}^\ell \sum_{c'\neq c} \left(\sum_{k=1}^{n_c}\frac{s_c}{n_c}y_{kc1}-\mu^*_{1, \text{DIM}}s_c \right) \left(\sum_{k=1}^{n_{c'}}\frac{s_{c'}}{n_{c'}}y_{kc'0}-\mu^*_{0, \text{DIM}}s_{c'} \right)
    \nn {}& \hspace{3ex} - \frac{1}{\left(\sum_{c=1}^\ell s_c\right)^2} \sum_{c=1}^\ell \left(\sum_{k=1}^{n_c}\frac{s_c}{n_c}y_{kc1}-\mu^*_{1, \text{DIM}}s_c \right)\left(\sum_{k=1}^{n_c}\frac{s_c}{n_c}y_{kc0}-\mu^*_{0, \text{DIM}}s_c \right) \label{dimcovmu}
\end{align}
The third equality occurs because units are sampled independently across clusters and that units in the same cluster are given the same treatments (i.~e., $\cov(S_{kc}, S_{k^*c'})=\cov(S_{kc}, S_{k'c}) = 0$).

\subsection{Linear transforms on DIM estimator for the population mean}

For any constants $a, b$,
\begin{align}
    \hat{\mu}_{t, \text{DIM,SRS}}(a+b\mathbf{y}) &= \frac{\sum_{c=1}^\ell S_cT_{ct}\sum_{c=1}^{n_c} (a+by_{kct})S_{kc}}{\sum_{c=1}^\ell S_cT_{ct}s_c}
    \nn &= \frac{\sum_{c=1}^\ell S_cT_{ct}\sum_{c=1}^{n_c} aS_{kc}}{\sum_{c=1}^\ell S_cT_{ct}s_c} + \frac{\sum_{c=1}^\ell S_cT_{ct}\sum_{c=1}^{n_c} by_{kct}S_{kc}}{\sum_{c=1}^\ell S_cT_{ct}s_c}
    \nn &=  a\frac{\sum_{c=1}^\ell S_cT_{ct}s_c}{\sum_{c=1}^\ell S_cT_{ct}s_c} + b\frac{\sum_{c=1}^\ell S_cT_{ct}\sum_{c=1}^{n_c} y_{kct}S_{kc}}{\sum_{c=1}^\ell S_cT_{ct}s_c}
    \nn &= a + b\hat{\mu}_{t, \text{DIM,SRS}}(\mathbf{y}) \label{dimlinearmu}
\end{align}

\subsection{Proof of lemma~\ref{dimlemma}} \label{dimlemmaproof}

Based on eq.~\eqref{dimexpmu}, the DIM estimator is biased for PATE:
\begin{align}
    \E(\hat\delta_\text{DIM,SRS}) ={}& \E(\hat\mu_{1,\text{DIM,SRS}})-\E(\hat\mu_{0,\text{DIM,SRS}})
    \nn ={}& \frac{1}{\sum_{c=1}^\ell s_c}\left[ \sum_{c=1}^\ell \sum_{k=1}^{n_c} \frac{s_c}{n_c} y_{kc1} - \frac{\ell}{\#T_1}\cov\left( \hat\mu_{1,\text{DIM, SRS}}, \sum_{c=1}^\ell S_cT_{c1}s_c \right) \right]
    \nn {}&- \frac{1}{\sum_{c=1}^\ell s_c}\left[ \sum_{c=1}^\ell \sum_{k=1}^{n_c} \frac{s_c}{n_c} y_{kc0} - \frac{\ell}{\#T_0}\cov\left( \hat\mu_{0,\text{DIM, SRS}}, \sum_{c=1}^\ell S_cT_{c0}s_c \right)\right]
    \nn =&{}  \frac{1}{\sum_{c=1}^\ell s_c}\left[ \sum_{c=1}^\ell \sum_{k=1}^{n_c} \frac{s_c}{n_c} (y_{kc1}-y_{kc0}) \right]
    \nn {}& - \frac{1}{\sum_{c=1}^\ell s_c}\frac{\ell}{\#T_1}\cov\left( \hat\mu_{1,\text{DIM, SRS}}, \sum_{c=1}^\ell S_cT_{c1}s_c 
    \right)
    \nn {}& +\frac{1}{\sum_{c=1}^\ell s_c} \frac{\ell}{\#T_0}\cov\left( \hat\mu_{0,\text{DIM, SRS}}, \sum_{c=1}^\ell S_cT_{c0}s_c 
    \right).
\end{align}

\noindent From eq.~\eqref{dimvarmu} and eq.~\eqref{dimcovmu}, the variance of the DIM estimator can be approximated by
\begin{align}
    \var(\hat\delta_\text{DIM,SRS}) \approx{}& \frac{\ell^2}{\left(\sum_{c=1}^\ell s_c\right)^2} \left[\E\left(\frac{1}{\#T_1}\right) - \frac{1}{\ell}\right] \var\left[\left(\tau^*_{c1}-\mu^*_{1,\text{DIM}}s_c\right)\right] 
    \nn {}& + \frac{\ell}{\left(\sum_{c=1}^\ell s_c\right)^2} \E\left(\frac{1}{\#T_1}\right) \sum_{c=1}^\ell s_c\left(1-\frac{s_c}{n_c}\right)\var(y_{kc1})
   \nn ={}& \frac{\ell^2}{\left(\sum_{c=1}^\ell s_c\right)^2} \left[\E\left(\frac{1}{\#T_0}\right) - \frac{1}{\ell}\right] \var\left[\left(\tau^*_{c0}-\mu^*_{0,\text{DIM}}s_c\right)\right] 
    \nn {}& + \frac{\ell}{\left(\sum_{c=1}^\ell s_c\right)^2} \E\left(\frac{1}{\#T_0}\right) \sum_{c=1}^\ell s_c\left(1-\frac{s_c}{n_c}\right)\var(y_{kc0})
    \nn {}& - \frac{2}{\left(\sum_{c=1}^\ell s_c\right)^2} \frac{1}{\ell-1} \sum_{c=1}^\ell \sum_{c'\neq c} \left(\sum_{k=1}^{n_c}\frac{s_c}{n_c}y_{kc1}-\mu^*_{1, \text{DIM}}s_c \right) \left(\sum_{k=1}^{n_{c'}}\frac{s_{c'}}{n_{c'}}y_{kc'0}-\mu^*_{0, \text{DIM}}s_{c'} \right)
    \nn {}& + \frac{2}{\left(\sum_{c=1}^\ell s_c\right)^2} \sum_{c=1}^\ell \left(\sum_{k=1}^{n_c}\frac{s_c}{n_c}y_{kc1}-\mu^*_{1, \text{DIM}}s_c \right)\left(\sum_{k=1}^{n_c}\frac{s_c}{n_c}y_{kc0}-\mu^*_{0, \text{DIM}}s_c \right).
\end{align}

\noindent Lastly, since $\hat\mu_{t,\text{DIM,SRS}}$ is linear [see eq.~\eqref{dimlinearmu}],
\begin{align}
    \hat\delta_\text{DIM,SRS}(a + \mathbf{y}) &= \hat\mu_{1,\text{DIM,SRS}}(a + \mathbf{y}) - \hat\mu_{0,\text{DIM,SRS}}(a + \mathbf{y})
    \nn &= \hat\delta_\text{DIM,SRS}.
\end{align}
