# Supplementary material for: The Benefits of Probability-Proportional-to-Size Sampling in Cluster-Randomized Experiments
Source: arXiv:2002.08009 source file (2020-02-19)
Supplement: Supplementary file 3 [file AppendixC-dr.tex]

\cleardoublepage

\section{Properties of the DR estimator} \label{appendixdr}

We begin by investigating the properties of $\hat\mu_{t,\text{DR,SRS}}$.  Then using these properties, we prove lemma~\ref{DRSRSlemma}.  

\subsection{Expectation of DR estimator for population mean} 

From eq.~\eqref{htexpmu},
\begin{align}
   \E(\mu_{t,\text{DR,SRS}}) &= \E\left(\ell \sum_{c=1}^\ell \frac{S_cT_{ct}}{\#T_t}\frac{n_c}{n}\left[\sum_{k=1}^{n_c}\frac{y_{kct}S_{kc}}{s_c}-\frac{\theta_t}{n_c}\left(n_c-\frac{n}{\ell}\right) \right] \right)
  \nn &= \E\left(\ell \sum_{c=1}^\ell \frac{S_cT_{ct}}{\#T_t}\frac{n_c}{n}\sum_{k=1}^{n_c}\frac{y_{kct}S_{kc}}{s_c}\right)-\E\left(\ell \sum_{c=1}^\ell \frac{S_cT_{ct}}{\#T_t}\frac{\theta_t}{n}\left[n_c-\frac{n}{\ell}\right] \right)
  \nn &= \mu_t - \ell\sum_{c=1}^\ell \frac{\theta_t}{n}\left(n_c-\frac{n}{\ell}\right) \E\left(\frac{S_cT_{ct}}{\#T_t}\right)
  \nn &= \mu_t - \sum_{c=1}^\ell \frac{\theta_t}{n}\left(n_c-\frac{n}{\ell}\right) = \mu_t \label{drexpmu}
\end{align}
 
\subsection{Variance of DR estimator for population mean} 

Note that
\begin{align}
    \hat \mu_{t,\text{DR,SRS}} &= \ell \sum_{c=1}^\ell \frac{S_cT_{ct}}{\#T_t}\frac{n_c}{n}\left[\sum_{k=1}^{n_c}\frac{y_{kct}S_{kc}}{s_c}-\frac{\theta_t}{n_c}\left(n_c-\frac{n}{\ell} \right) \right]\\
  &= \ell \sum_{c=1}^\ell \frac{S_cT_{ct}}{\#T_t}\frac{n_c}{n}\hat{\Tilde\mu}_{ct},
\end{align}
which has the same form as the HT estimator.  Hence, based on eq.~\eqref{htvarmu}, the variance of $\hat\mu_{t,\text{DR,SRS}}$ is
\begin{equation}
     \var(\hat\mu_{t,\text{DR},\text{SRS}}) = \ell^2 \left[\E\left(\frac{1}{\#T_t}\right)-\frac{1}{\ell} \right]\var\left(\frac{n_c}{n}\Tilde\mu_{ct}\right) + \E\left(\frac{1}{\#T_t}\right) \ell \sum_{c=1}^\ell \frac{n_c^2}{n^2}\left(1-\frac{s_c}{n_c}\right)\frac{\var(y_{kct})}{s_c}
    \label{drvarmu}
\end{equation}
where $\var\left(\frac{n_c}{n}\tilde\mu_{ct}\right)$ is the population variance of the weighted transformed treatment means $\tilde\mu_{ct}=\mu_{ct}-\frac{\theta_t}{n_c}(n_c-\frac{n}{\ell})$ and $\var(y_{kct})$ is the population variance of within-cluster outcomes under treatment $t$.

\subsection{Covariance of DR estimator for the population means}

From eq.~\eqref{dericovHT},
\begin{equation}
    \cov(\hat\mu_{1,\text{DR},\text{SRS}}, \hat\mu_{0,\text{DR},\text{SRS}}) = \frac{\ell}{\ell-1} \sum\limits_{c=1}^\ell \sum\limits_{c\neq c'} \frac{n_cn_{c'}}{n^2} \tilde\mu_{c1} \tilde\mu_{c'0} - \mu_1\mu_0.
\label{drcovmu} 
\end{equation}

\subsection{Linear transforms on DR estimator for the population mean}

For any constants $a, b$,
\begin{align}
    \hat\mu_{t,\text{DR,SRS}}(a+b\mathbf{y}) &= \ell \sum_{c=1}^\ell \frac{S_cT_{ct}}{\#T_t}\frac{n_c}{n}\left[\sum_{k=1}^{n_c}\frac{(a + by_{kct})S_{kc}}{s_c}-\frac{(a + b\theta_t)}{n_c}\left(n_c-\frac{n}{\ell} \right) \right]
   \nn &= \ell \sum_{c=1}^\ell \frac{S_cT_{ct}}{\#T_t}\frac{n_c}{n} \left[a - \frac{a}{n_c}\left(n_c-\frac{n}{\ell}\right)  + \sum_{k=1}^{n_c}\frac{by_{kct}S_{kc}}{s_c}-\frac{b\theta_t}{n_c}\left(n_c-\frac{n}{\ell}\right)\right]
   \nn &= a\sum_{c=1}^\ell \frac{S_cT_{ct}}{\#T_t} + b\hat\mu_{t,\text{DR,SRS}}
   \nn &= a + b\hat\mu_{t,\text{DR,SRS}}(\mathbf{y}) \label{drlinearmu}
\end{align}

\subsection{Proof of lemma~\ref{DRSRSlemma}} \label{drlemmaproof}

Since $\hat\mu_{t,\text{DR,SRS}}$ is unbiased for $\mu_t$ [see eq.~\eqref{drexpmu}],
\begin{align}
    \E(\hat\delta_\text{DR,SRS}) &= \E(\hat\mu_{1,\text{DR,SRS}})-\E(\hat\mu_{0,\text{DR,SRS}})
    \nn &= \mu_1 - \mu_0 = \delta.
\end{align}
From eq.~\eqref{drvarmu} and eq.~\eqref{drcovmu},
\begin{align}
    \var(\hat\delta_\text{DR,SRS}) ={}& \ell^2 \left[\E\left(\frac{1}{\#T_1}\right)-\frac{1}{\ell} \right]\var\left(\frac{n_c}{n}\Tilde\mu_{c1}\right) + \E\left(\frac{1}{\#T_1}\right) \ell \sum_{c=1}^\ell \frac{n_c^2}{n^2}\left(1-\frac{s_c}{n_c}\right)\frac{\var(y_{kc1})}{s_c} 
    \nn {}& + \ell^2 \left[\E\left(\frac{1}{\#T_0}\right)-\frac{1}{\ell} \right]\var\left(\frac{n_c}{n}\Tilde\mu_{c0}\right) + \E\left(\frac{1}{\#T_0}\right) \ell \sum_{c=1}^\ell \frac{n_c^2}{n^2}\left(1-\frac{s_c}{n_c}\right)\frac{\var(y_{kc0})}{s_c} 
    \nn {}& - 2\frac{\ell}{\ell-1} \sum\limits_{c=1}^\ell \sum\limits_{c\neq c'} \frac{n_cn_{c'}}{n^2} \tilde\mu_{c1} \tilde\mu_{c'0} + 2 \mu_1\mu_0.
\end{align}

\noindent Finally, based on eq.~\eqref{drlinearmu}, the DR estimator for PATE is location-invariant since
\begin{align}
    \hat\delta_\text{DR,SRS}(a + \mathbf{y}) &= \hat\mu_{1,\text{DR,SRS}}(a + \mathbf{y}) - \hat\mu_{0,\text{DR,SRS}}(a + \mathbf{y})
    \nn &= \hat\delta_\text{DR,SRS}.
\end{align}

\subsection{Expectation of DR estimator with estimated $\theta$}

If $\theta$ is unknown and needs to be estimated with the data,
\begin{align}
    \E(\hat{\mu}_{t,\text{DR}}) &= \mu_t - \ell \sum_{c=1}^\ell \frac{1}{n}\left(n_c - \frac{n}{\ell} \right) \E\left(\frac{S_cT_{ct}\hat\theta}{\#T_t}\right)
    \nn &= \mu_t - \ell \sum_{c=1}^\ell \frac{1}{n}\left(n_c - \frac{n}{\ell} \right) \left[ \cov\left(\frac{S_cT_{ct}}{\#T_t}, \hat\theta\right) - \E\left(\frac{S_cT_{ct}}{\#T_t}\right)\E(\hat\theta) \right]
    \nn &= \mu_t - \ell \sum_{c=1}^\ell \frac{1}{n}\left(n_c - \frac{n}{\ell} \right) \cov\left(\frac{S_cT_{ct}}{\#T_t}, \hat\theta\right) + \sum_{c=1}^\ell \frac{1}{n}\left(n_c - \frac{n}{\ell} \right) \E(\hat\theta)
    \nn &= \mu_t - \ell \sum_{c=1}^\ell \frac{1}{n}\left(n_c - \frac{n}{\ell} \right) \cov\left(\frac{S_cT_{ct}}{\#T_t}, \hat\theta\right).
\end{align}
Therefore,
\begin{align}
    \E(\hat\delta_\text{DR,SRS}) ={}& \delta - \ell \sum_{c=1}^\ell \frac{1}{n}\left(n_c - \frac{n}{\ell} \right) \cov\left(\frac{S_cT_{c1}}{\#T_1}, \hat\theta\right) 
    \nn {}& + \ell \sum_{c=1}^\ell \frac{1}{n}\left(n_c - \frac{n}{\ell} \right) \cov\left(\frac{S_cT_{c0}}{\#T_0}, \hat\theta\right).
\end{align}
